# Supplementary material for: Intriguing Properties of Modern GANs
Source: arXiv:2402.14098 source file (2024-02-21)
Supplement: Supplementary file 1 [file OD_IN_AFHQ.tex]

\begin{figure}
\begin{center}
    \includegraphics[width=.8\textwidth]{supp_figures/OD_IN_AFHQ.pdf}
\end{center}
  \caption{The GANs' performance on OD in ImageNet10, AFHQCat and AFHQDog, compared to the performance of the baselines.}
  \label{fig:app-OD-AFHQ}

\end{figure}
