# Supplementary material for: Intriguing Properties of Modern GANs
Source: arXiv:2402.14098 source file (2024-02-21)
Supplement: Supplementary file 2 [file avg_OD.tex]

\begin{figure}
\begin{center}
    \includegraphics[width=.8\textwidth]{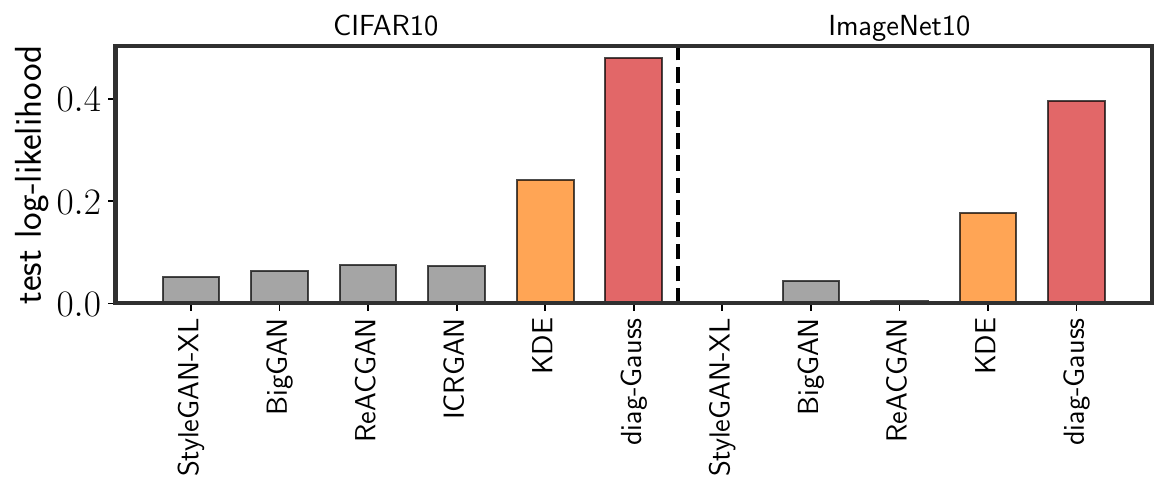}
\end{center}
  \caption{OD results when averaging over all labels. Here, again, the baseline models outperform the GANs investigated.}
  \label{fig:app-avg-OD}

\end{figure}
