# Supplementary material for: Intriguing Properties of Modern GANs
Source: arXiv:2402.14098 source file (2024-02-21)
Supplement: Supplementary file 3 [file other_norms.tex]

\begin{figure}
\begin{center}
    \includegraphics[width=.8\textwidth]{supp_figures/other_norms.pdf}
\end{center}
  \caption{Classification (top) and OD (bottom) performance for various different distance functions. The GANs perform poorly with all distance functions explored.}
  \label{fig:app-other-norms}

\end{figure}
